# Supplementary material for: UniTalker: Scaling up Audio-Driven 3D Facial Animation through A Unified Model
Source: arXiv:2408.00762 source file (2024-08-01)
Supplement: Supplementary file 1 [file 0_overview.tex]

\section{Overview}
% Give an overview of the Supp

This supplementary materials provide additional information regarding the related works, model design, experiment results and the limitations of this work.

In section \ref{sec:supp_related_works_dataset}, we introduce the distinctions and connections between vertex-based annotations and parameter-based facial motion annotations. We introduce the conventional re-topology technique, which transforms meshes from one topology to another using linear transformations. This elucidates our rationale for selecting a linear layer as the decoder head in our model. 
In section \ref{sec:supp_related_works_regression_autoregression}, we review the utilization of autoregressive and regressive models in recent studies focusing on audio-driven 3D facial motion. 
In section \ref{sec:supp_IPCA_and_DW}, we investigate the feasibility of implementing the decoder warm-up strategy independently, without the need for adopting the IPCA strategy. We discuss more functionality of IPCA in this section. 
In section \ref{sec:supp_PIE}, we discuss more on the pivot identity embedding (PIE) strategy. Additionally, we explore alternative solutions to address the issue of dataset bias leakage.
In section \ref{sec:supp_dataset_description}, we show the details of the datasets used in the experiments. 
In section \ref{sec:supp_experiment_details}, we show the details of the experimental settings. 
In section \ref{sec:supp_frequency_adaptor_position}, we present a comparative analysis of various position choices of the frequency adaptor.
In section \ref{sec:dataset_contribution_analysis}, we present additional analysis focusing on the contribution of different datasets to the overall model performance. This analysis aims to clarify the importance of incorporating mixed datasets to train a foundation model.
In section \ref{sec:supp_transfer_to_tiny},  we showcase UniTalker's ability to transfer to unseen annotation conventions, even with minimal training data, including just a few audio-visual pairs or even one pair.
% 
% we show more results on annotation transfer to demonstrate the necessity of mixed datasets to build a foundation model. Firstly, we show that tuning the decoder part of the UniTalker-L-[D0-D7] model on a single dataset yields better performance that directly training the model on the dataset does. Secondly, to show that tuning a UniTalker model on an unseen dataset can greatly reduce the requirement of data size, we tune the decoder of UniTalker-L-[D1-D7] on D0 dataset and show the precision to data size relation. Thirdly, we utilise the mini-dataset transfer method explained in Section \missref to demonstrate that our model can transfer to new conventions with extremely small dataset. We show the visual results in the attached video.
% 
In section \ref{sec:supp_user_study}, we present a user study that qualitatively compares our work with previous state-of-the-art approaches.
In section \ref{sec:supp_future_work}, we expose the limitations of UniTalker and outline future plans to address them.
